# Supplementary material for: T-STAR: Truthful Style Transfer using AMR Graph as Intermediate Representation
Source: arXiv:2212.01667 source file (2022-12-03)
Supplement: Supplementary file 1 [file case-stydy-appendix.tex]

\begin{table*}
\centering
\resizebox{1\textwidth}{!}{%
\begin{tabular} {|p{2.5cm}|p{4.3cm}|p{4.3cm}|p{4.3cm}|p{2cm}|}
\hline
\textbf{Styles} & \textbf{Input Sentence} & \textbf{\textit{STRAP}} &  \textbf{\textit{GIST}} & \textbf{Category}\\ 
\hline 
\textit{Poetry -\textgreater Bible} & Look on the hands with female slaughter red; & And see now the blood of the \textcolor{red}{woman's hands upon the hands of the man}. & Look unto the redness of the hands of the female slaughter. & Semantic Drift\\
\textit{Poetry -\textgreater Bible} & Lifted his curved lids, and kept them wide & And he lifted up his broad lid, and laid it open upon \textcolor{red}{the carcase of the lamb}. & He hath lifted up his curvy lid, and kept it wide. & Hallucinates \\
\textit{Poetry -\textgreater Shak.} & But weep, and weep, that they were born so fair? & But cry out, and weep, \textcolor{red}{That men’s blood should be so sweetly grown?} & But weep at being so fair borne?  & Hallucinates\\
\textit{Switch -\textgreater Shak.} & oh yes Jessica Tandy won best actress and uh say  & Jessica Tandy had \textcolor{red}{her best performance} & Jessica Tandy won best actress, and thou say’st she is & Semantic Drift \\
\textit{Switch -\textgreater Shak.} & no i don't think so because uh i saw just a little bit of the game today and he was out there playing  & No, I know not because that, sir, I saw a little play of this \textcolor{red}{yesterday} and he played \textcolor{red}{his king to ’t.} & Not to think so, for I have seen just a little bit of game today, and he’s playing out there. & Semantic Drift \\
\textit{Switch -\textgreater Shak.} & yeah i'm again- i'm against this uh automatic and semiautomatic stuff i don't think we should have access to those  & Against automatic and semiautomatic \textcolor{red}{weapons} I do not think we should have access & ea, yeah, I am against this automatic and semiautomatic stuff And think not we should have access to that stuff. & Halluciates \\
\textit{Bible -\textgreater Switch.} & The trees of the LORD are full of sap; the cedars of Lebanon, which he hath planted & God planted a lot of trees \textcolor{red}{for the Lord's trees} he was out in the cedars of Lebanon he uh & Lord's trees are full of sap and the Lebanon cedars that he planted & Incomplete \\
\textit{Bible -\textgreater Switch.} &  And Abraham gave all that he had unto Isaac. & 
Isaac \textcolor{red}{Isaac and Abraham} were giving everything away & and Abraham gave Isaac all he had &  Semantic Drift \\
\textit{Switch. -\textgreater Bible} &  what kind of meals did she make that you liked & and what manner of things did ye desire?  & What kind of meal will she make that ye like?  & Incomplete \\
\hline 
\end{tabular}}
\caption{Case Study. Example of generated style transfer sentences for STRAP and GIST models.}
\label{tab:case-study-appendix}
\end{table*}

\begin{table*}
\centering
\resizebox{1\textwidth}{!}{%
\begin{tabular} {|p{2.5cm}|p{4.3cm}|p{4.3cm}|p{4.3cm}|}
\hline
\textbf{Styles} & \textbf{Input Sentence} & \textbf{\textit{STRAP}} &  \textbf{\textit{GIST}}\\ 
\hline 
\textit{Shak. -\textgreater Bible} & But if you do, sir, I am for you. 
 & And he said unto them, If thou wilt walk in my ways, I will be with thee  &  But if he do, I will support him. \\
\textit{Shak. -\textgreater Poetry} & Talk not to me, for I’ll not speak a word & And speak not of me; I'll not speak, & Talk not to me, for I will not speak a word. 
 \\ \hline
 \textit{Shak. -\textgreater Switch} & Talk not to me, for I’ll not speak a word & don't you know i'm not going to talk & not talk to me i'm not going to speak the word  \\ \hline
 \textit{Poetry -\textgreater Bible} & A wretch! a villain! lost to love and truth!  & A fool, a man of destruction, forsaken in love and truth! &  The wretch, and the villain, and the lost in love and truth; \\ \hline
 \textit{Switch to Shak.} & yeah nice talking to you  & I am glad to hear you speak with me. & It were nice talking with you. \\
 \hline
\end{tabular}}
\caption{Case Study. Examples where GIST does not perform efficient style transfer as compared to the baseline.}
\label{tab:limitations-appendix}
\end{table*}
